# Supplementary material for: In Silico Seawater
Source: arXiv:2401.13158 source file (2024-01-24)
Supplement: Supplementary file 1 [file seawater_SI.pdf]

**Supporting Information to paper entitled**  
**“In Silico” Seawater**

Ivan M. Zeron, Miguel A. Gonzalez, Edoardo Errani, Carlos Vega, and Jose L. F. Abascal

*Departamento de Química Física, Facultad de Ciencias Químicas,  
Universidad Complutense de Madrid, 28040 Madrid, Spain*

## OPTIMIZED SOLUTE SAMPLES FOR MOLECULAR SIMULATIONS

The Reference Composition of “Standard Seawater” was defined<sup>1</sup> in terms of the mole fractions of the 15 major components based on the most accurate prior determinations of the composition. The stoichiometry was adjusted to achieve charge balance by making use of the 2005 atomic weights and finally rounded to 7 digits after the decimal point. Taking into account that the number of water molecules at the usual seawater salinities is about 50 times the total number of solute molecules, the sample required to match the Reference Composition would be of the order of  $5 \times 10^8$  molecules. This is a prohibitive number for a molecular simulation run. It is then necessary to simplify the stoichiometry. In this work we made the assumption that a system considering only the six more abundant constituents could be able to account for the physico-chemical properties of seawater. These solutes (all of them are ionic compounds) represent a 99.7 percent of the mole fraction and the remainder 0.3 needs to be explicitly considered because it mostly corresponds to negatively charged molecules. Thus, we grouped together these minor components assigning them a single negative charge.

The procedure to obtain a simplified sample is simple in principle. We may obtain more or less representative samples by multiplying the Reference Composition mole fractions by a factor and converting the resulting results to integer numbers. However, the real to integer numbers conversion distorts the input stoichiometry and, even more importantly, does not guarantee the charge neutrality of the sample. After analyzing the ratios between the relative abundance of the constituents and a considerable trial and error we arrived at a composition made of 318 ions that reproduced the Reference Composition of Standard Seawater with a root mean square deviation of only 0.0003. The agreement for a such a reduced sample is quite extraordinary so the finding was probably a lucky event not extendible to more complex samples. We thus decided to carry a systematic search of samples with optimal composition.

The first step of the procedure is to choose a number of constituents. For instance, if we intend to consider explicitly only the ions whose mole fraction is greater than that of bicarbonate we fix this number to six. For a given set of components and total sample size we calculate the number of molecules of each type according to the mole fractions defined in the Reference Composition,  $x_{ref}$  and round them to the nearest integers. For example, for sample sizes of 300 and 1000 solutes we obtain (146.2, 125.6, 14.2, 7.6, 2.8, 2.7) and (487.5, 418.8, 47.2, 25.2, 9.2, 9.1), respectively, for the six major components, yielding (146, 126, 14, 8, 3, 3) and (487, 419, 47, 25, 9, 9) ions when rounded to the nearest integers. Notice that these samples are not electrically neutral. We then define a new type of component (labeled as “Others” in Table I) and assign it the mole fraction needed to get a total mole fraction

of 1 ( $x_{others} = 0.00303$  when including explicitly 6 solutes). The number of molecules of this special solute type and its charge are calculated to ensure that the sample is electrically balanced. In our examples above, the number of “Others” molecules would be 1 and 3, carrying a single negative charge (i.e., that of the chloride anion) in both cases. Using these numbers we calculate the actual mole fractions of the proposed samples. A reasonable measure of the quality of the sample is the root mean square of the deviations, *rmsd*, between the calculated and the reference mole fractions. These amount to 0.00175 and 0.00034 for 300 and 1000 ions, respectively.

As shown in the example above, increasing the sample size usually improves the agreement between the stoichiometry of the simplified seasalt sample and that of the Reference Composition. However, there are sample sizes that produce a closer agreement with a reduced number of ions. For instance, a sample of 318 ions leads to  $rmsd = 0.00034$ , five times smaller than that for 300 solute molecules and identical to that obtained for a 1000 ions sample. Thus, 318 ions should be considered an optimal choice for systems considering explicitly six components. We have carried out a systematic scanning of the sample sizes considering different number of components. Some of the resulting optimal samples are presented in Table I. There we use the notation  $ISSS_{m,n}$ , where ISSS is the acronym of “in silico” sea salt,  $m$  is the total number of solute molecules and  $n$  is the number of constituents explicitly included (the rest of components are grouped together as “Others”). Curiously, some sizes are optimal for different number of constituents. For instance,  $ISSS_{1313,n}$  is optimal for  $n = 6$  (not shown in Table I because  $ISSS_{1631,6}$  is even better), 7 and 8.

Several factors limit effectively the use of a large number of components to represent the stoichiometry of seawater. The first one is the size of the system when water molecules are added to the seasalt composition. For normal ocean salinities a minimum of 15, 63, 193 and 630 thousands of molecules are required to include explicitly 6, 8, 10 and 13 components, respectively. But apart of the burden of generating initial configurations for the largest samples, the molecular simulation of these systems could be affordable. Molecular dynamics programs usually require small amounts of memory and larger system sizes allow to obtain statistically acceptable quantities with shorter simulation times. However, to ensure an equilibrated system the diffusion of the ions should allow, in principle, to explore many different ionic environments.

It is very likely that the preceding assertion would not be a real shortcoming in practice. Let us assume that we are interested in the determination of, for instance, the diffusivity of the fluoride ion in seawater. According to Table I an optimal sample for a salinity  $S = 35.165$  g/kg would be made of 629705 water and 13166 solute molecules. Among the latter, there would be just one strontium ion. Certainly, ensuring that the interactions between the single strontium and fluoride ions are statistically sampled would be an extremely costly

task. But a poor sampling of these interactions has an almost null impact in the diffusivity of the fluoride ion. It is clear that the effect of replacing the interactions of a single ion (strontium) by a another one with similar interatomic potential would be much smaller than the statistical uncertainty of the calculated diffusion coefficient even for extremely long simulations. The same argument would probably be extensive to bicarbonate (only 20 ions in a sample of 630 thousand molecules!).

In fact, the main factor limiting the number of solutes explicitly included in the ISSS stoichiometry seems to be the availability of an accurate forcefield for the components. In the example above, instead of using a very detailed seasalt composition, it would be advisable to tune carefully the interactions of the fluoride anion with the most abundant seawater components, i.e. water, chloride and sodium. In the extreme case of the “Others” molecules such availability is impossible by definition. In order to look for optimal samples we need at least to assign them a charge. The neglected solutes in the ISSS<sub>*m,n*</sub> samples with  $n = 6, 8$  are mostly anions so we attribute them a negative charge. For  $n = 10, 13$  the global charge of the excluded solutes is more or less balanced and we thus assume them to be neutral molecules.

TABLE I. Optimized samples producing a close agreement with the Reference Composition of seasalt<sup>1</sup> using a reduced number of solute molecules. The upper row shows the total number of solute molecules (designed as ions for simplicity) in the sample. The columns labeled  $n$  and  $x$  are the number of ions and the corresponding mole fraction of each one. The latter may be compared with the mole fractions defined in the Reference Composition,  $x_{ref}$ . The root mean square of the deviations  $x - x_{ref}$  for each sample is given in the row denoted as  $rmsd$ . The last row indicates the number of water molecules for a salinity  $S = 35.165$  g/kg.

| Notation           |           | ISSS <sub>318,6</sub> | ISSS <sub>1631,6</sub> | ISSS <sub>1313,7</sub> | ISSS <sub>3371,7</sub> | ISSS <sub>1313,8</sub> | ISSS <sub>5871,8</sub> | ISSS <sub>4047,10</sub> | ISSS <sub>14480,10</sub> | ISSS <sub>13166,13</sub> | ISSS <sub>61313,13</sub> |
|--------------------|-----------|-----------------------|------------------------|------------------------|------------------------|------------------------|------------------------|-------------------------|--------------------------|--------------------------|--------------------------|
| #ions              |           | 318                   | 1631                   | 1313                   | 3371                   | 1313                   | 5871                   | 4047                    | 14480                    | 13166                    | 61313                    |
|                    | $x_{ref}$ | $n$ $x$               | $n$ $x$                | $n$ $x$                | $n$ $x$                | $n$ $x$                | $n$ $x$                | $n$ $x$                 | $n$ $x$                  | $n$ $x$                  | $n$ $x$                  |
| Chloride           | 0.4874839 | 155 0.48742           | 795 0.48743            | 640 0.48743            | 1643 0.48739           | 640 0.48743            | 2862 0.48748           | 1973 0.48752            | 7059 0.48750             | 6418 0.48747             | 29889 0.48748            |
| Sodium             | 0.4188071 | 133 0.41824           | 683 0.41876            | 550 0.41889            | 1412 0.41887           | 550 0.41889            | 2459 0.41884           | 1695 0.41883            | 6064 0.41878             | 5514 0.41881             | 25678 0.41880            |
| Magnesium          | 0.0471678 | 15 0.04717            | 77 0.04721             | 62 0.04722             | 159 0.04717            | 62 0.04722             | 277 0.04718            | 191 0.04720             | 683 0.04717              | 621 0.04717              | 2892 0.04717             |
| Sulfate            | 0.0252152 | 8 0.02516             | 41 0.02514             | 33 0.02513             | 85 0.02522             | 33 0.02513             | 148 0.02521            | 102 0.02520             | 365 0.02521              | 332 0.02522              | 1546 0.02521             |
| Calcium            | 0.0091823 | 3 0.00943             | 15 0.00920             | 12 0.00914             | 31 0.00920             | 12 0.00914             | 54 0.00920             | 37 0.00914              | 133 0.00919              | 121 0.00919              | 563 0.00918              |
| Potassium          | 0.0091159 | 3 0.00943             | 15 0.00920             | 12 0.00914             | 31 0.00920             | 12 0.00914             | 54 0.00920             | 37 0.00914              | 132 0.00912              | 120 0.00911              | 559 0.00912              |
| Bicarbonate        | 0.0015340 |                       |                        | 2 0.00152              | 5 0.00148              | 2 0.00152              | 9 0.00153              | 6 0.00148               | 22 0.00152               | 20 0.00152               | 94 0.00153               |
| Bromide            | 0.0007520 |                       |                        |                        |                        | 1 0.00076              | 4 0.00068              | 3 0.00074               | 11 0.00076               | 10 0.00076               | 46 0.00075               |
| Boric acid         | 0.0002807 |                       |                        |                        |                        |                        |                        | 1 0.00025               | 4 0.00028                | 4 0.00030                | 17 0.00028               |
| Carbonate          | 0.0002134 |                       |                        |                        |                        |                        |                        | 1 0.00025               | 3 0.00021                | 3 0.00023                | 13 0.00021               |
| Borate             | 0.0000900 |                       |                        |                        |                        |                        |                        |                         |                          | 1 0.00008                | 6 0.00010                |
| Strontium          | 0.0000810 |                       |                        |                        |                        |                        |                        |                         |                          | 1 0.00008                | 5 0.00008                |
| Fluoride           | 0.0000610 |                       |                        |                        |                        |                        |                        |                         |                          | 1 0.00008                | 4 0.00007                |
| Others             | 0.0000157 | 1 0.00314             | 5 0.00307              | 2 0.00152              | 5 0.00148              | 1 0.00076              | 4 0.00068              | 1 0.00025               | 4 0.00028                | 0 0.00000                | 1 0.00002                |
| $rmsd \times 10^4$ |           | 3.4                   | 0.9                    | 0.9                    | 0.6                    | 0.8                    | 0.5                    | 0.5                     | 0.15                     | 0.14                     | 0.03                     |
| #water             |           | 15210                 | 78004                  | 62792                  | 161223                 | 62786                  | 280751                 | 193541                  | 692558                   | 629705                   | 2932449                  |

---

<sup>1</sup> F. J. Millero, R. Feistel, D. G. Wright, and T. J. McDougall, Deep Sea Research I **55**, 50 (2008).
